# Supplementary material for: PoTATO: A Dataset for Analyzing Polarimetric Traces of Afloat Trash Objects
Source: arXiv:2409.12659 source file (2024-09-19)
Supplement: Supplementary file 1 [file X_suppl.tex]

\section{Code Availability and Reproducibility}
\label{sec:code}

All code used for the extraction of visualizations from RAW images, including the training of the object detection models and the generation of metrics and statistics presented in this paper, is accessible in the anonymous repository.%
\footnote{Available at \url{https://anonymous.4open.science/r/PoTATO-62B4/README.md}} Detailed instructions to reproduce the results are provided in the \texttt{README.md} file and all specific library versions are listed in the \texttt{requirements.txt} file.

\section{Dataset Content and Availability}
While logistical challenges limited dataset expansion, we ensured meticulous recording. Each experiment consists of multiple short clips as shown in Figure \ref{fig:sequence_graph}. In between them, bottles were approached from different directions and repositioned to other areas of the lake, ensuring diverse backgrounds and wide range of lighting conditions due to relative sun position. Even within the same sequence, the bottle distance to the boat changes significantly (Figure \ref{fig:sequence_images}) altering the bounding box size and covering regions with different polarimetric properties. Our dataset has substantial variability in the polarimetric information despite being collected in a single location. 

\begin{figure}[bh]
\centering
\begin{subfigure}{0.4\linewidth}
    \centering
    \includegraphics[width=\linewidth]{img/sequence_graph.png}
    \caption{Experiment 7 has 50 different clips.}
    \label{fig:sequence_graph}
\end{subfigure}
\hfill % This adds space between the two subfigures
\begin{subfigure}{0.55\linewidth}
    \centering
    \includegraphics[width=\linewidth]{img/sequence_images.jpg}
    \caption{Change in Relative Bottle Position}
    \label{fig:sequence_images}
\end{subfigure}

\caption{Temporal Analysis of Image Sequence.}
\label{fig:sequence}
\end{figure}

The dataset is compressed into the \texttt{potato.tgz} file, with a size of $16.08GB$. It includes RAW format images along with labels in both COCO and YOLO formats. The train, validation, and test splits utilized during the evaluation are accessible as a list of file names in text files. Supplementary to the dataset, images from a calibration board are included. The calibration board features a $9\times7$ checkerboard pattern, with each square measuring $108$ millimeters. Captured at distances ranging from 1 to 8 meters, these images enable the estimation of intrinsic calibration parameters if needed.

\begin{figure}[bth]
\begin{center}
\includegraphics[width=\linewidth]{img/size-position.png}
\end{center}
   \caption{ Correlation between bounding box size and its position in the image plane}
\label{fig:image_position}
\end{figure}

Larger bounding boxes have stronger polarimetric signals due to perspective geometry as explained in Subsection \ref{subsec:advantages}. Also, given the fixed camera position in the vessel, closer objects will appear lower in the image plane. Figure \ref{fig:image_position} offers further clarification on the distribution of bounding box sizes, highlighting their correlation with the vertical position on the image plane.

Attached we present the video \textit{test\_set\_overview.mov} providing a visual representation and insights into the performance disparities among different channels. The video includes image sequences from the test set, where ground truth labels are indicated by green bounding boxes along with the output of the trained Faster CNN object detection model. 
Link to the full dataset is available in our laboratory website.

\section{Additional Images}

This section supplements the experiments with four additional figures illustrating the effectiveness of POL and DIF images techniques in enhancing contrast and filtering reflections in scenarios involving water surfaces and objects like bottles. Specifically, it demonstrates how POL images reveal distinct polarization angles, improving object-background contrast, while DIF images are effective in filtering out reflections, even in conditions of intense light polarization or when objects blend with background patterns like water ripples.

\begin{figure*}[bth]
\begin{center}
\includegraphics[width=\linewidth]{img/exp05_frame023893_tile.jpg}
\end{center}
   \caption{Bottles concealed in background reflection in the RGB image and with stronger contrast in the POL image}
\label{fig:eg_exp05}
\end{figure*}

\begin{figure*}[bth]
\begin{center}
\includegraphics[width=\linewidth]{img/exp07_frame022868_tile.jpg}
\end{center}
   \caption{DOLP image indicating the region closer to the vessel with strong polarimetric signals.
   The DIF image filters out reflections from intense light polarization. Simultaneously, a POL image increases the contrast between a bottle and the background in the right side. }
\label{fig:eg_exp07_1}
\end{figure*}

\begin{figure*}[bth]
\begin{center}
\includegraphics[width=\linewidth]{img/exp07_frame053098_tile.jpg}
\end{center}
   \caption{A floating bottle that looks similar to ripples on water surface in the RGB image and its contrast is highlighted on POL image with different AoLP.}
\label{fig:eg_exp07_2}
\end{figure*}

\begin{figure*}[bth]
\begin{center}
\includegraphics[width=\linewidth]{img/exp03_frame00273_tile.jpg}
\end{center}
   \caption{Captured under a clear sky, the water reflects the skylight's polarization patterns. The DIF image is capable of reducing the reflection also when the angle of polarization is not horizontal. Such a result is unattainable when using a fixed linear polarization filter.}
\label{fig:eg_exp03}
\end{figure*}
